# Supplementary material for: Traffic Flow Optimisation for Lifelong Multi-Agent Path Finding
Source: arXiv:2308.11234 source file (2024-01-31)
Supplement: Supplementary file 1 [file appendix.tex]

\newpage
\clearpage
% \appendix
% \appendixpage

\begin{table}[t]
\centering
\caption{APX-EXP-1; Results on Warehouse}
\begin{tabular}{lll}
\toprule
                  ALG & Throughput & RT (s) \\
\midrule
            GP-R100 &   23.6±5.8 &        0.18±0.083 \\
         GP-NO-R100 &   21.9±5.5 &       0.175±0.086 \\
    GP-SUM-OVC-R100 &   22.9±5.7 &        0.17±0.083 \\
   GP-SUM-NOVC-R100 &   17.0±4.6 &       0.136±0.081 \\
   GP-SUI\_TC-R100 &   20.0±5.2 &       0.076±0.029 \\
GP-SUI\_TC-R100-F1.2 &   21.8±5.5 &       0.107±0.044 \\
  GP-SUI\_TC-R100-F2 &   21.9±5.5 &       0.149±0.069 \\
     GP-SUI\_TG-R100 &   19.3±5.1 &       0.064±0.038 \\
            PIBT &   19.3±5.0 &       0.021±0.092 \\
\bottomrule
\end{tabular}
\label{tab:add-w}
\end{table}

\begin{table}[t]
\centering
\caption{APX-EXP-1; Results on Sortation}
\begin{tabular}{lll}
\toprule
                  ALG & Throughput & RT (s) \\
\midrule
            GP-R100 &   10.9±3.5 &       0.004±0.002 \\
         GP-NO-R100 &    9.9±3.3 &       0.003±0.002 \\
    GP-SUM-OVC-R100 &   11.8±3.8 &       0.003±0.002 \\
   GP-SUM-NOVC-R100 &    9.5±3.3 &       0.003±0.002 \\
   GP-SUI\_TC-R100 &    8.8±3.1 &       0.002±0.001 \\
GP-SUI\_TC-R100-F1.2 &   11.0±3.6 &       0.002±0.001 \\
  GP-SUI\_TC-R100-F2 &   11.2±3.6 &       0.003±0.002 \\
     GP-SUI\_TG-R100 &    8.5±3.1 &       0.002±0.001 \\
            PIBT &    6.2±2.6 &         0.001±0.0 \\
\bottomrule
\end{tabular}
\label{tab:add-s}

\end{table}

\begin{table}[t]
\centering
\caption{APX-EXP-1; Results on Game}
\begin{tabular}{lll}
\toprule
                  ALG & Throughput & RT (s) \\
\midrule
            GP-R100 &   45.7±8.6 &       0.153±0.041 \\
         GP-NO-R100 &   45.4±8.5 &       0.152±0.041 \\
    GP-SUM-OVC-R100 &   46.5±8.7 &       0.138±0.037 \\
   GP-SUM-NOVC-R100 &   43.2±8.1 &       0.129±0.037 \\
    GP-SUI\_TC-R100 &   44.3±8.4 &        0.06±0.015 \\
GP-SUI\_TC-R100-F1.2 &   45.7±8.5 &       0.077±0.019 \\
  GP-SUI\_TC-R100-F2 &   45.6±8.5 &       0.124±0.032 \\
     GP-SUI\_TG-R100 &   41.7±8.0 &       0.048±0.012 \\
            PIBT &   41.9±7.7 &       0.015±0.065 \\
\bottomrule
\end{tabular}
\label{tab:add-g}
\end{table}

\begin{table}
\centering
\caption{APX-EXP-1; Results on Room}
\begin{tabular}{lll}
\toprule
                  ALG & Throughput & RT (s) \\
\midrule
            GP-R100 &    2.2±1.5 &       0.003±0.006 \\
         GP-NO-R100 &    2.4±1.6 &       0.003±0.006 \\
    GP-SUM-OVC-R100 &    3.1±1.8 &       0.003±0.005 \\
   GP-SUM-NOVC-R100 &    2.9±1.7 &       0.003±0.005 \\
   GP-SUI\_TC-R100 &    2.7±1.6 &       0.002±0.002 \\
GP-SUI\_TC-R100-F1.2 &    2.9±1.7 &       0.002±0.002 \\
  GP-SUI\_TC-R100-F2 &    3.1±1.8 &       0.003±0.005 \\
     GP-SUI\_TG-R100 &    2.7±1.7 &       0.002±0.002 \\
            PIBT &    2.8±1.7 &       0.001±0.002 \\
\bottomrule
\end{tabular}
\label{tab:add-r}
\end{table}

\section*{Appendix}

We report results from supplementary experiments to further highlight the strengths of Guided PIBT. First, we consider other variants of Guided PIBT, with alternative formulations for the heuristic and results with the traffic-aware SU-I heuristic of~\cite{han2022optimizing}, which we mentioned in the main paper as a related work.
We also compare results vs. RHCR~\cite{li2021lifelong}, a leading but less scalable approach for lifelong MAPF. 

\subsection*{APX-EXP-1: Variants of Guided PIBT}

Guided PIBT is a flexible framework for deriving high-quality move actions using guide path and PIBT.
Practitioners can adjust the objective function for computing the guide path when planning on different domains. 
Table~\ref{tab:add-w}, Table~\ref{tab:add-s}, Table~\ref{tab:add-g} and Table~\ref{tab:add-r} each shows results for different variants of Guided PIBT on Table~\ref{tab: heiristic} experiment setting, as follows:
\begin{itemize}
    \item \texttt{GP-NO} Normalize  \emph{contraflow cost} $\hat{c}_e = c_e / n$, where $n = f_{v_1,v_2} + f_{v_2,v_1}, e \equiv (v_1, v_2) \in E$. In corridors, contraflow costs increase exponentially for Guided PIBT. The normalized \emph{contraflow cost} by comparison calculates the potential increase per agent and tests if it improves the solution on maps with fewer corridors.
    \item \texttt{GP-SUM-OVC} using the sum of congestion costs $1 + c_e + p_v$ as objective for guide path planning. This approach compares our suggested strict traffic order method with a sum-of-congestion-costs model that may balance path length and traffic congestion avoidance.
    \item \texttt{GP-SUM-NOVC} using the $1 + \hat{c}_e + p_v$ as objective for guide path planning. Same motivation for \texttt{GP-SUM-OVC} but using normalized \emph{contraflow cost} instead.
    \item \texttt{GP-SUI\_TC} using SU-I cost-to-come \cite{han2022optimizing} congestion cost to compute guide path. The existing study suggests adding SU-I cost-to-come congestion cost on the action cost (the sum of congestion cost along a path is guaranteed smaller than 1) to compute optimal length paths that tie-breaks towards smaller congestion cost. We examine the effectiveness of this method for guiding PIBT. 
    \item \texttt{GP-SUI\_TG} \citet{han2022optimizing} also suggest SU-I cost-to-go heuristic to avoid traffic congestion, which adds a congestion score (between 0 and 1) to heuristics as a tie-breaker. We examine the effectiveness of it for computing guide path for lifelong MAPF (previous work considers only one-shot MAPF). 
    \item \texttt{GP-SUI\_TC-F$x$} the original SU-I cost-to-come and cost-to-go heuristic only acts as a tie-breaker, and is limited to the optimal path. Here we search for the SU-I cost-to-come minimized path within the bound of $C* \times x$.
    % \item \texttt{THV-R100-OA} using vertex cost minimized heuristic but only update heuristics for agents receiving new tasks at each timestep, the initialisation is relaxed to 100 heuristics per timestep.
    % For THV-R100-OA, the results for warehouse and game is not out yet, the results on small maps are similar to THV-R100.
    
\end{itemize}
